# Supplementary material for: Learning Constraints and Descriptive Segmentation for Subevent Detection
Source: arXiv:2109.06316 source file (2021-09-13)
Supplement: Supplementary file 1 [file 7appendix.tex]

\section{Appendices}
\label{sec:appendix}
